# Supplementary material for: Parity nonconserving interactions of electrons in chiral molecules with cosmic fields
Source: arXiv:2005.03938 ancillary file (2020-05-08)
Supplement: Supplementary file 1 [file suppl.pdf]

# Supplemantary Material to *Parity nonconserving interactions of electrons in chiral molecules with cosmic fields*

Konstantin Gaul,[1] Mikhail G. Kozlov,[2,3] Timur A. Isaev,[2] and Robert Berger[1]

[1]*Fachbereich Chemie, Philipps-Universität Marburg, Hans-Meerwein-Straße 4, 35032 Marburg, Germany*

[2]*Petersburg Nuclear Physics Institute of NRC "Kurchatov Institute", Gatchina 188300, Russia*

[3]*St. Petersburg Electrotechnical University "LETI", Prof. Popov Str. 5, 197376 St. Petersburg*

(Dated: May 8, 2020)

In the following, we list numerical data that is plotted in different figures of the paper *Parity nonconserving interactions of electrons in chiral molecules with cosmic fields.*

Data for the dihedral angle dependence of $\left\langle \hat{H}_{\mathrm{ew}} \right\rangle$ in $H_2Po_2$ and $H_2O_2$ differ slightly from those presented in Ref. [1] due to the choice of a different basis set.

The one-dimensional cut through the multi-dimensional parity violating potential energy surface of $\left\langle \hat{H}_{\mathrm{ew}} \right\rangle$ along the dimensionless reduced normal coordinate ($q_4$) corresponding to the C–F stretching mode for the ($S$)-enantiomer of CHBrClF is a recalculation of that in Ref. [2]. Parameters for the polynomial fit of this one-dimensional cut can be found in Ref. [2].

[1] R. Berger, N. Langermann, and C. van Wüllen, Phys. Rev. A **71**, 042105 (2005).
[2] R. Berger and J. L. Stuber, Mol. Phys. **105**, 41 (2007).

Table I. Dihedral angle $\phi$ dependence of $\langle \boldsymbol{\gamma}^5 \rangle$ and $\left\langle \hat{H}_{\mathrm{ew}} \right\rangle$ for the compounds $H_2Po_2$ and $H_2O_2$. Negative values of $\phi$ correspond to the $(M)$-enantiomer, positive values of $\phi$ correspond to the $(P)$-enantiomer. Due to the use of a different basis set the values differ slightly from those in Ref. [1].

| $\phi/^\circ$ | $H_2O_2$ | | $H_2Po_2$ | |
|---|---|---|---|---|
| | $\langle \boldsymbol{\gamma}^5 \rangle \times 10^9$ | $\left\langle \hat{H}_{\mathrm{ew}} \right\rangle \times 10^{19}/E_{\mathrm{h}}$ | $\langle \boldsymbol{\gamma}^5 \rangle \times 10^4$ | $\left\langle \hat{H}_{\mathrm{ew}} \right\rangle \times 10^{12}/E_{\mathrm{h}}$ |
| −180 | ( 0.000003) | (0.00000005) | (0.0000001) | (0.0000007) |
| −170 | 2.07 | −2.97 | 0.84 | −0.54 |
| −160 | 3.88 | −5.58 | 1.54 | −0.99 |
| −150 | 5.21 | −7.51 | 2.00 | −1.27 |
| −140 | 5.92 | −8.55 | 2.17 | −1.37 |
| −130 | 5.91 | −8.60 | 2.08 | −1.29 |
| −120 | 5.20 | −7.69 | 1.76 | −1.06 |
| −110 | 3.93 | −5.94 | 1.27 | −0.72 |
| −100 | 2.29 | −3.58 | 0.67 | −0.31 |
| −90 | 0.41 | −0.87 | 0.02 | 0.14 |
| −80 | −1.62 | 1.87 | −0.63 | 0.61 |
| −70 | −3.66 | 4.36 | −1.22 | 0.94 |
| −60 | −5.51 | 6.30 | −1.71 | 1.25 |
| −50 | −6.75 | 7.45 | −2.03 | 1.44 |
| −40 | −7.04 | 7.67 | −2.14 | 1.49 |
| −30 | −6.35 | 6.89 | −1.99 | 1.37 |
| −20 | −4.82 | 5.20 | −1.55 | 1.06 |
| −10 | −2.62 | 2.80 | −0.85 | 0.58 |
| 0 | (0.0000005) | (-0.00000005) | (0.0000002) | (-0.0000004) |
| 10 | 2.62 | −2.80 | 0.85 | −0.58 |
| 20 | 4.82 | −5.20 | 1.55 | −1.06 |
| 30 | 6.35 | −6.89 | 1.99 | −1.37 |
| 40 | 7.04 | −7.67 | 2.14 | −1.49 |
| 50 | 6.75 | −7.45 | 2.03 | −1.44 |
| 60 | 5.51 | −6.30 | 1.71 | −1.25 |
| 70 | 3.66 | −4.36 | 1.22 | −1.04 |
| 80 | 1.62 | −1.87 | 0.63 | −0.61 |
| 90 | 0.41 | 0.87 | 0.02 | −0.14 |
| 100 | −2.29 | 3.58 | −0.67 | 0.31 |
| 110 | −3.93 | 5.94 | −1.27 | 0.72 |
| 120 | −5.20 | 7.69 | −1.76 | 1.06 |
| 130 | −5.91 | 8.60 | −2.08 | 1.29 |
| 140 | −5.92 | 8.55 | −2.17 | 1.37 |
| 150 | −5.21 | 7.51 | −2.00 | 1.27 |
| 160 | −3.88 | 5.58 | −1.54 | 0.99 |
| 170 | −2.07 | 2.97 | −0.84 | 0.54 |
| 180 | (0.00001) | (0.000002) | (0.00000003) | (-0.000002) |

Table II. One dimensional cut through the parity violating potential of $\left\langle \hat{H}_{\mathrm{ew}} \right\rangle$ and of $\langle \gamma^5 \rangle$ along the dimensionless reduced normal coordinate ($q_1$) corresponding to the C–H stretching mode for the ($S$)-enantiomer of CHBrClF.

| $q_1$ | $\langle \gamma^5 \rangle \times 10^9$ | | | $\left\langle \hat{H}_{\mathrm{ew}} \right\rangle \times 10^{17}/E_{\mathrm{h}}$ | | |
|---|---|---|---|---|---|---|
| | HF | B3LYP | LDA | HF | B3LYP | LDA |
| −3.000 | −3.873 | −10.908 | −15.102 | −0.649 | −0.302 | 0.047 |
| −2.500 | −3.478 | −10.598 | −14.799 | −0.655 | −0.278 | 0.087 |
| −2.000 | −3.102 | −10.261 | −14.434 | −0.660 | −0.256 | 0.124 |
| −1.500 | −2.810 | −9.899 | −14.019 | −0.663 | −0.236 | 0.158 |
| −1.000 | −2.556 | −9.496 | −13.551 | −0.665 | −0.216 | 0.189 |
| −0.500 | −2.278 | −9.027 | −13.007 | −0.665 | −0.197 | 0.217 |
| −0.250 | −2.156 | −8.760 | −12.698 | −0.664 | −0.188 | 0.231 |
| −0.125 | −2.065 | −8.617 | −12.532 | −0.663 | −0.183 | 0.237 |
| 0.000 | −1.978 | −8.461 | −12.360 | −0.662 | −0.179 | 0.243 |
| 0.125 | −1.914 | −8.312 | −12.178 | −0.661 | −0.174 | 0.249 |
| 0.250 | −1.828 | −8.149 | −11.989 | −0.660 | −0.169 | 0.255 |
| 0.500 | −1.634 | −7.804 | −11.586 | −0.657 | −0.160 | 0.267 |
| 1.000 | −1.221 | −7.037 | −10.680 | −0.650 | −0.142 | 0.289 |
| 1.500 | −0.778 | −6.174 | −9.638 | −0.641 | −0.124 | 0.309 |
| 2.000 | −0.301 | −5.217 | −8.454 | −0.629 | −0.107 | 0.327 |
| 2.500 | 0.206 | −4.145 | −7.112 | −0.615 | −0.089 | 0.343 |
| 3.000 | 0.776 | −2.917 | −5.577 | −0.598 | −0.072 | 0.357 |

Table III. One dimensional cut through the parity violating potential of $\left\langle \hat{H}_{\mathrm{ew}} \right\rangle$ and of $\langle \gamma^5 \rangle$ along the dimensionless reduced normal coordinate ($q_2$) corresponding to a H deformation mode for the ($S$)-enantiomer of CHBrClF.

| $q_2$ | $\langle \gamma^5 \rangle \times 10^9$ | | | $\left\langle \hat{H}_{\mathrm{ew}} \right\rangle \times 10^{17}/E_{\mathrm{h}}$ | | |
|---|---|---|---|---|---|---|
| | HF | B3LYP | LDA | HF | B3LYP | LDA |
| −3.000 | −35.802 | −42.051 | −43.518 | 0.992 | 1.367 | 1.641 |
| −2.500 | −31.382 | −36.544 | −37.496 | 0.793 | 1.194 | 1.492 |
| −2.000 | −26.313 | −30.629 | −31.421 | 0.557 | 0.980 | 1.301 |
| −1.500 | −20.746 | −24.723 | −25.765 | 0.288 | 0.729 | 1.073 |
| −1.000 | −14.824 | −19.057 | −20.746 | −0.007 | 0.448 | 0.817 |
| −0.500 | −8.563 | −13.666 | −16.333 | −0.325 | 0.144 | 0.538 |
| −0.250 | −5.329 | −11.050 | −14.303 | −0.492 | −0.016 | 0.392 |
| −0.125 | −3.661 | −9.755 | −13.322 | −0.577 | −0.097 | 0.318 |
| 0.000 | −1.978 | −8.461 | −12.360 | −0.662 | −0.179 | 0.243 |
| 0.125 | −0.305 | −7.186 | −11.413 | −0.749 | −0.261 | 0.168 |
| 0.250 | 1.423 | −5.908 | −10.480 | −0.836 | −0.345 | 0.092 |
| 0.500 | 4.916 | −3.365 | −8.651 | −1.013 | −0.513 | −0.061 |
| 1.000 | 12.146 | 1.668 | −5.117 | −1.375 | −0.856 | −0.371 |
| 1.500 | 19.614 | 6.573 | −1.754 | −1.745 | −1.204 | −0.681 |
| 2.000 | 27.204 | 11.266 | 1.375 | −2.121 | −1.553 | −0.988 |
| 2.500 | 34.980 | 15.732 | 4.254 | −2.501 | −1.902 | −1.288 |
| 3.000 | 42.788 | 20.095 | 6.976 | −2.885 | −2.248 | −1.580 |

Table IV. One dimensional cut through the parity violating potential of $\left\langle \hat{H}_{\mathrm{ew}} \right\rangle$ and of $\langle \boldsymbol{\gamma}^5 \rangle$ along the dimensionless reduced normal coordinate ($q_3$) corresponding to a H deformation mode for the ($S$)-enantiomer of CHBrClF.

| $q_3$ | $\langle \boldsymbol{\gamma}^5 \rangle \times 10^9$ | | | $\left\langle \hat{H}_{\mathrm{ew}} \right\rangle \times 10^{17}/E_\mathrm{h}$ | | |
|---|---|---|---|---|---|---|
| | HF | B3LYP | LDA | HF | B3LYP | LDA |
| −3.000 | −54.412 | −57.731 | −68.613 | 0.983 | 1.761 | 2.414 |
| −2.500 | −39.591 | −46.409 | −57.416 | 0.690 | 1.414 | 2.028 |
| −2.000 | −27.193 | −36.853 | −47.533 | 0.407 | 1.082 | 1.658 |
| −1.500 | −17.211 | −28.536 | −38.322 | 0.131 | 0.758 | 1.295 |
| −1.000 | −9.790 | −21.118 | −29.410 | −0.140 | 0.439 | 0.938 |
| −0.500 | −4.832 | −14.443 | −20.713 | −0.405 | 0.126 | 0.586 |
| −0.250 | −3.205 | −11.370 | −16.481 | −0.535 | −0.027 | 0.413 |
| −0.125 | −2.536 | −9.898 | −14.405 | −0.599 | −0.103 | 0.328 |
| 0.000 | −1.978 | −8.461 | −12.360 | −0.662 | −0.179 | 0.243 |
| 0.125 | −1.522 | −7.079 | −10.347 | −0.725 | −0.253 | 0.160 |
| 0.250 | −1.123 | −5.730 | −8.372 | −0.787 | −0.327 | 0.077 |
| 0.500 | −0.479 | −3.145 | −4.536 | −0.910 | −0.472 | −0.086 |
| 1.000 | 0.651 | 1.661 | 2.662 | −1.146 | −0.748 | −0.395 |
| 1.500 | 2.333 | 6.191 | 9.324 | −1.367 | −1.004 | −0.678 |
| 2.000 | 5.156 | 10.761 | 15.741 | −1.571 | −1.235 | −0.931 |
| 2.500 | 9.361 | 15.724 | 22.370 | −1.757 | −1.440 | −1.151 |
| 3.000 | 14.944 | 21.425 | 29.706 | −1.925 | −1.617 | −1.337 |

Table V. One dimensional cut through the parity violating potential of $\left\langle \hat{H}_{\mathrm{ew}} \right\rangle$ and of $\langle \boldsymbol{\gamma}^5 \rangle$ along the dimensionless reduced normal coordinate ($q_4$) corresponding to the C–F stretching mode for the ($S$)-enantiomer of CHBrClF. Recalculated values of $\left\langle \hat{H}_{\mathrm{ew}} \right\rangle$ are indentical to those in Ref. [2].

| $q_4$ | $\langle \boldsymbol{\gamma}^5 \rangle \times 10^9$ | | | | $\left\langle \hat{H}_{\mathrm{ew}} \right\rangle \times 10^{17}/E_\mathrm{h}$ | | | |
|---|---|---|---|---|---|---|---|---|
| | HF | B3LYP | BLYP | LDA | HF | B3LYP | BLYP | LDA |
| −3.00 | 1.552 | −9.451 | −11.373 | −16.689 | −1.405 | −0.923 | −0.586 | −0.465 |
| −2.50 | 0.529 | −9.736 | −11.351 | −16.430 | −1.260 | −0.783 | −0.460 | −0.331 |
| −2.00 | −0.294 | −9.796 | −11.092 | −15.935 | −1.122 | −0.649 | −0.340 | −0.204 |
| −1.50 | −0.937 | −9.667 | −10.639 | −15.245 | −0.993 | −0.521 | −0.226 | −0.083 |
| −1.00 | −1.420 | −9.381 | −10.033 | −14.398 | −0.873 | −0.400 | −0.118 | 0.032 |
| −0.50 | −1.762 | −8.970 | −9.310 | −13.426 | −0.763 | −0.286 | −0.015 | 0.141 |
| −0.25 | −1.885 | −8.726 | −8.915 | −12.903 | −0.711 | −0.231 | 0.033 | 0.193 |
| −0.125 | −1.935 | −8.596 | −8.710 | −12.634 | −0.687 | −0.205 | 0.057 | 0.218 |
| 0.00 | −1.978 | −8.461 | −8.502 | −12.360 | −0.662 | −0.179 | 0.081 | 0.243 |
| 0.125 | −2.014 | −8.321 | −8.290 | −12.082 | −0.639 | −0.153 | 0.104 | 0.268 |
| 0.25 | −2.042 | −8.177 | −8.075 | −11.799 | −0.616 | −0.128 | 0.126 | 0.292 |
| 0.50 | −2.079 | −7.877 | −7.637 | −11.223 | −0.571 | −0.079 | 0.170 | 0.339 |
| 1.00 | −2.075 | −7.237 | −6.735 | −10.034 | −0.490 | 0.012 | 0.254 | 0.427 |
| 1.50 | −1.972 | −6.556 | −5.811 | −8.803 | −0.417 | 0.096 | 0.330 | 0.507 |
| 2.00 | −1.772 | −5.842 | −4.870 | −7.533 | −0.354 | 0.172 | 0.399 | 0.580 |
| 2.50 | −1.476 | −5.096 | −3.910 | −6.220 | −0.299 | 0.240 | 0.461 | 0.645 |
| 3.00 | −1.085 | −4.317 | −2.925 | −4.858 | −0.253 | 0.301 | 0.516 | 0.701 |

Table VI. One dimensional cut through the parity violating potential of $\left\langle \hat{H}_{\mathrm{ew}} \right\rangle$ and of $\langle \gamma^5 \rangle$ along the dimensionless reduced normal coordinate ($q_5$) corresponding to the C–Cl stretching mode for the ($S$)-enantiomer of CHBrClF.

| $q_5$ | $\langle \gamma^5 \rangle \times 10^9$ | | | $\left\langle \hat{H}_{\mathrm{ew}} \right\rangle \times 10^{17}/E_{\mathrm{h}}$ | | |
|---|---|---|---|---|---|---|
| | HF | B3LYP | LDA | HF | B3LYP | LDA |
| −3.000 | −9.682 | −38.716 | −53.160 | 0.205 | 1.082 | 1.815 |
| −2.500 | −8.372 | −32.636 | −44.684 | −0.001 | 0.766 | 1.422 |
| −2.000 | −7.138 | −26.939 | −36.818 | −0.182 | 0.494 | 1.084 |
| −1.500 | −5.857 | −21.622 | −29.579 | −0.339 | 0.264 | 0.798 |
| −1.000 | −4.516 | −16.718 | −23.025 | −0.472 | 0.075 | 0.564 |
| −0.500 | −3.209 | −12.301 | −17.247 | −0.580 | −0.072 | 0.379 |
| −0.250 | −2.593 | −10.305 | −14.685 | −0.624 | −0.130 | 0.305 |
| −0.125 | −2.283 | −9.365 | −13.491 | −0.644 | −0.156 | 0.273 |
| 0.000 | −1.978 | −8.461 | −12.360 | −0.662 | −0.179 | 0.243 |
| 0.125 | −1.716 | −7.613 | −11.291 | −0.679 | −0.199 | 0.217 |
| 0.250 | −1.441 | −6.805 | −10.288 | −0.694 | −0.217 | 0.193 |
| 0.500 | −0.947 | −5.332 | −8.486 | −0.718 | −0.245 | 0.154 |
| 1.000 | −0.220 | −3.018 | −5.758 | −0.747 | −0.272 | 0.110 |
| 1.500 | 0.073 | −1.652 | −4.282 | −0.748 | −0.260 | 0.108 |
| 2.000 | −0.219 | −1.349 | −4.175 | −0.720 | −0.211 | 0.147 |
| 2.500 | −1.246 | −2.219 | −5.515 | −0.661 | −0.126 | 0.223 |
| 3.000 | −3.154 | −4.351 | −8.360 | −0.571 | −0.007 | 0.332 |

Table VII. One dimensional cut through the parity violating potential of $\left\langle \hat{H}_{\mathrm{ew}} \right\rangle$ and of $\langle \gamma^5 \rangle$ along the dimensionless reduced normal coordinate ($q_6$) corresponding to the C–Br stretching mode for the ($S$)-enantiomer of CHBrClF.

| $q_6$ | $\langle \gamma^5 \rangle \times 10^9$ | | | $\left\langle \hat{H}_{\mathrm{ew}} \right\rangle \times 10^{17}/E_{\mathrm{h}}$ | | |
|---|---|---|---|---|---|---|
| | HF | B3LYP | LDA | HF | B3LYP | LDA |
| −3.000 | 1.256 | 23.994 | 33.867 | −1.149 | −1.258 | −1.256 |
| −2.500 | −0.534 | 16.251 | 22.471 | −1.048 | −1.022 | −0.928 |
| −2.000 | −1.492 | 9.723 | 12.893 | −0.956 | −0.811 | −0.634 |
| −1.500 | −1.907 | 4.200 | 4.879 | −0.873 | −0.624 | −0.373 |
| −1.000 | −1.976 | −0.537 | −1.832 | −0.796 | −0.457 | −0.141 |
| −0.500 | −1.929 | −4.696 | −7.498 | −0.726 | −0.309 | 0.063 |
| −0.250 | −1.937 | −6.620 | −10.015 | −0.694 | −0.242 | 0.156 |
| −0.125 | −1.964 | −7.552 | −11.207 | −0.678 | −0.210 | 0.201 |
| 0.000 | −1.978 | −8.461 | −12.360 | −0.662 | −0.179 | 0.243 |
| 0.125 | −2.043 | −9.369 | −13.474 | −0.647 | −0.148 | 0.285 |
| 0.250 | −2.106 | −10.257 | −14.555 | −0.632 | −0.119 | 0.325 |
| 0.500 | −2.307 | −12.004 | −16.622 | −0.603 | −0.063 | 0.401 |
| 1.000 | −3.010 | −15.413 | −20.439 | −0.548 | 0.038 | 0.538 |
| 1.500 | −4.161 | −18.746 | −23.902 | −0.496 | 0.126 | 0.656 |
| 2.000 | −5.744 | −21.996 | −27.038 | −0.449 | 0.202 | 0.757 |
| 2.500 | −7.684 | −25.100 | −29.813 | −0.405 | 0.267 | 0.842 |
| 3.000 | −9.935 | −27.951 | −32.142 | −0.364 | 0.322 | 0.912 |

Table VIII. One dimensional cut through the parity violating potential of $\left\langle \hat{H}_{\mathrm{ew}} \right\rangle$ and of $\left\langle \boldsymbol{\gamma}^5 \right\rangle$ along the dimensionless reduced normal coordinate ($q_7$) corresponding to the Cl–F deformation mode for the ($S$)-enantiomer of CHBrClF.

| $q_7$ | $\left\langle \boldsymbol{\gamma}^5 \right\rangle \times 10^9$ | | | $\left\langle \hat{H}_{\mathrm{ew}} \right\rangle \times 10^{17}/E_{\mathrm{h}}$ | | |
|---|---|---|---|---|---|---|
| | HF | B3LYP | LDA | HF | B3LYP | LDA |
| −3.000 | 2.661 | 15.056 | 20.305 | −2.229 | −2.190 | −2.012 |
| −2.500 | 1.995 | 10.349 | 13.674 | −1.981 | −1.837 | −1.613 |
| −2.000 | 0.942 | 6.017 | 7.618 | −1.710 | −1.492 | −1.223 |
| −1.500 | 0.042 | 2.010 | 2.055 | −1.443 | −1.153 | −0.843 |
| −1.000 | −0.766 | −1.715 | −3.087 | −1.179 | −0.821 | −0.472 |
| −0.500 | −1.440 | −5.196 | −7.874 | −0.918 | −0.496 | −0.110 |
| −0.250 | −1.728 | −6.856 | −10.151 | −0.790 | −0.337 | 0.068 |
| −0.125 | −1.869 | −7.668 | −11.264 | −0.726 | −0.257 | 0.156 |
| 0.000 | −1.978 | −8.461 | −12.360 | −0.662 | −0.179 | 0.243 |
| 0.125 | −2.122 | −9.256 | −13.439 | −0.599 | −0.100 | 0.330 |
| 0.250 | −2.236 | −10.033 | −14.503 | −0.536 | −0.022 | 0.416 |
| 0.500 | −2.449 | −11.554 | −16.587 | −0.410 | 0.132 | 0.587 |
| 1.000 | −2.817 | −14.473 | −20.588 | −0.163 | 0.435 | 0.921 |
| 1.500 | −3.096 | −17.233 | −24.381 | 0.080 | 0.731 | 1.245 |
| 2.000 | −3.298 | −19.834 | −27.967 | 0.318 | 1.018 | 1.560 |
| 2.500 | −3.412 | −22.267 | −31.339 | 0.550 | 1.297 | 1.863 |
| 3.000 | −3.459 | −24.515 | −34.475 | 0.776 | 1.567 | 2.155 |

Table IX. One dimensional cut through the parity violating potential of $\left\langle \hat{H}_{\mathrm{ew}} \right\rangle$ and of $\left\langle \boldsymbol{\gamma}^5 \right\rangle$ along the dimensionless reduced normal coordinate ($q_8$) corresponding to the Br–F deformation mode for the ($S$)-enantiomer of CHBrClF.

| $q_8$ | $\left\langle \boldsymbol{\gamma}^5 \right\rangle \times 10^9$ | | | $\left\langle \hat{H}_{\mathrm{ew}} \right\rangle \times 10^{17}/E_{\mathrm{h}}$ | | |
|---|---|---|---|---|---|---|
| | HF | B3LYP | LDA | HF | B3LYP | LDA |
| −3.000 | 11.097 | 61.469 | 84.571 | −2.506 | −2.862 | −2.985 |
| −2.500 | 8.517 | 50.044 | 69.095 | −2.202 | −2.433 | −2.475 |
| −2.000 | 6.114 | 38.520 | 53.341 | −1.897 | −1.997 | −1.954 |
| −1.500 | 3.883 | 26.912 | 37.325 | −1.591 | −1.554 | −1.422 |
| −1.000 | 1.796 | 15.222 | 21.049 | −1.284 | −1.104 | −0.879 |
| −0.500 | −0.150 | 3.437 | 4.497 | −0.974 | −0.645 | −0.324 |
| −0.250 | −1.092 | −2.498 | −3.891 | −0.819 | −0.413 | −0.042 |
| −0.125 | −1.535 | −5.478 | −8.114 | −0.740 | −0.296 | 0.100 |
| 0.000 | −1.978 | −8.461 | −12.360 | −0.662 | −0.179 | 0.243 |
| 0.125 | −2.432 | −11.467 | −16.626 | −0.584 | −0.060 | 0.387 |
| 0.250 | −2.881 | −14.476 | −20.915 | −0.505 | 0.058 | 0.532 |
| 0.500 | −3.772 | −20.529 | −29.564 | −0.347 | 0.298 | 0.824 |
| 1.000 | −5.495 | −32.794 | −47.170 | −0.028 | 0.784 | 1.418 |
| 1.500 | −7.232 | −45.318 | −65.246 | 0.296 | 1.282 | 2.028 |
| 2.000 | −9.034 | −58.164 | −83.867 | 0.625 | 1.793 | 2.654 |
| 2.500 | −10.888 | −71.404 | −103.117 | 0.960 | 2.318 | 3.297 |
| 3.000 | −12.911 | −85.116 | −123.090 | 1.303 | 2.858 | 3.960 |

Table X. One dimensional cut through the parity violating potential of $\left\langle \hat{H}_{\mathrm{ew}} \right\rangle$ and of $\left\langle \gamma^5 \right\rangle$ along the dimensionless reduced normal coordinate ($q_9$) corresponding to the Br–Cl deformation mode for the ($S$)-enantiomer of CHBrClF.

| $q_9$ | $\left\langle \gamma^5 \right\rangle \times 10^9$ | | | $\left\langle \hat{H}_{\mathrm{ew}} \right\rangle \times 10^{17}/E_\mathrm{h}$ | | |
|---|---|---|---|---|---|---|
| | HF | B3LYP | LDA | HF | B3LYP | LDA |
| −3.000 | −19.015 | −40.759 | −54.207 | −0.241 | 0.396 | 0.888 |
| −2.500 | −16.245 | −35.655 | −47.676 | −0.312 | 0.299 | 0.778 |
| −2.000 | −13.423 | −30.408 | −40.917 | −0.382 | 0.202 | 0.669 |
| −1.500 | −10.565 | −25.044 | −33.971 | −0.452 | 0.106 | 0.561 |
| −1.000 | −7.691 | −19.586 | −26.872 | −0.522 | 0.011 | 0.454 |
| −0.500 | −4.826 | −14.053 | −19.659 | −0.592 | −0.084 | 0.348 |
| −0.250 | −3.409 | −11.266 | −16.018 | −0.627 | −0.131 | 0.296 |
| −0.125 | −2.701 | −9.868 | −14.191 | −0.645 | −0.155 | 0.270 |
| 0.000 | −1.978 | −8.461 | −12.360 | −0.662 | −0.179 | 0.243 |
| 0.125 | −1.296 | −7.065 | −10.524 | −0.680 | −0.202 | 0.217 |
| 0.250 | −0.589 | −5.660 | −8.685 | −0.698 | −0.226 | 0.191 |
| 0.500 | 0.807 | −2.846 | −5.002 | −0.733 | −0.274 | 0.139 |
| 1.000 | 3.521 | 2.794 | 2.386 | −0.806 | −0.369 | 0.034 |
| 1.500 | 6.136 | 8.438 | 9.785 | −0.879 | −0.466 | −0.072 |
| 2.000 | 8.652 | 14.071 | 17.175 | −0.954 | −0.564 | −0.178 |
| 2.500 | 11.087 | 19.690 | 24.541 | −1.031 | −0.664 | −0.285 |
| 3.000 | 13.350 | 25.282 | 31.771 | −1.110 | −0.766 | −0.395 |

Table XI. Resulting parameters of the polynomial fit to the one dimensional cut through the parity violating potential due to $\left\langle \gamma^5 \right\rangle$ along the dimensionless reduced normal coordinate ($q_1$) corresponding to the C–H stretching mode for the ($S$)-enantiomer of CHBrClF. The standard uncertainties resulting from the fit procedure are given in parenthesis in units of the last preceeding one or two digits.

| $k$ | $c_{\gamma^5,k} \times 10^9$ | | | $c_{\mathrm{ew},k} \times 10^{18}/E_\mathrm{h}$ | | |
|---|---|---|---|---|---|---|
| | HF | B3LYP | LDA | HF | B3LYP | LDA |
| 0 | −1.982(5) | −8.461(3) | −12.354(3) | −6.622 09(12) | −1.785 54(7) | 2.433 19(6) |
| 1 | 0.646(5) | 1.210(3) | 1.419(3) | 0.071 84(12) | 0.366 23(7) | 0.497 68(6) |
| 2 | 0.087(4) | 0.188(2) | 0.231(2) | 0.046 17(9) | −0.005 22(5) | −0.043 81(4) |
| 3 | 0.0144(8) | 0.0133(5) | 0.0188(4) | 0.001 357(19) | 0.001 893(11) | 0.002 094(9) |
| 4 | −0.0044(5) | −0.0018(3) | −0.0009(2) | −0.000 372(11) | −0.000 432(6) | −0.000 284(5) |

Table XII. Resulting parameters of the polynomial fit to the one dimensional cut through the parity violating potential due to $\left\langle \gamma^5 \right\rangle$ along the dimensionless reduced normal coordinate ($q_2$) corresponding to the H deformation mode for the ($S$)-enantiomer of CHBrClF. The standard uncertainties resulting from the fit procedure are given in parenthesis in units of the last preceeding one or two digits.

| $k$ | $c_{\gamma^5,k} \times 10^9$ | | | $c_{\mathrm{ew},k} \times 10^{18}/E_\mathrm{h}$ | | |
|---|---|---|---|---|---|---|
| | HF | B3LYP | LDA | HF | B3LYP | LDA |
| 0 | −1.976(16) | −8.43(3) | −12.32(5) | −6.6219(16) | −1.7850(10) | 2.4338(11) |
| 1 | 13.573(16) | 10.47(4) | 7.89(5) | −6.8816(17) | −6.5817(10) | −6.0084(11) |
| 2 | 0.612(12) | −0.33(2) | −0.68(3) | −0.2864(12) | −0.2541(8) | −0.2030(8) |
| 3 | −0.052(2) | −0.010(5) | 0.062(7) | 0.0467(2) | 0.062 13(16) | 0.071 36(17) |
| 4 | −0.0006(14) | 0.005(3) | 0.002(4) | −0.003 28(14) | −0.004 12(9) | −0.003 72(10) |

Table XIII. Resulting parameters of the polynomial fit to the one dimensional cut through the parity violating potential due to $\langle\gamma^5\rangle$ along the dimensionless reduced normal coordinate ($q_3$) corresponding to the H deformation mode for the ($S$)-enantiomer of CHBrClF. The standard uncertainties resulting from the fit procedure are given in parenthesis in units of the last preceeding one or two digits.

| $k$ | $c_{\gamma^5,k} \times 10^9$ | | | $c_{\mathrm{ew},k} \times 10^{18}/E_\mathrm{h}$ | | |
|---|---|---|---|---|---|---|
| | HF | B3LYP | LDA | HF | B3LYP | LDA |
| 0 | −2.05(14) | −8.50(5) | −12.39(10) | −6.621(5) | −1.785(9) | 2.433(11) |
| 1 | 4.90(14) | 11.01(5) | 15.65(10) | −5.036(5) | −5.945(9) | −6.680(11) |
| 2 | −2.47(10) | −1.19(3) | −0.95(7) | 0.190(3) | 0.235(6) | 0.278(8) |
| 3 | 0.75(2) | 0.238(7) | 0.072(15) | 0.0214(7) | 0.0359(13) | 0.0487(17) |
| 4 | 0.057(12) | 0.014(4) | 0.019(9) | 0.0024(4) | 0.0048(8) | 0.0056(9) |

Table XIV. Resulting parameters of the polynomial fit to the one dimensional cut through the parity violating potential due to $\langle\gamma^5\rangle$ along the dimensionless reduced normal coordinate ($q_4$) corresponding to the C–F stretching mode for the ($S$)-enantiomer of CHBrClF. For corresponding fit parameters of $\left\langle \hat{H}_\mathrm{ew} \right\rangle$ see the supplement of Ref. [2]. The standard uncertainties resulting from the fit procedure are given in parenthesis in units of the last preceeding one or two digits.

| $k$ | $c_{\gamma^5,k} \times 10^9$ | | | |
|---|---|---|---|---|
| | HF | B3LYP | BLYP | LDA |
| 0 | −1.9758(3) | −8.4609(8) | −8.4991(8) | −12.3571(7) |
| 1 | −0.3133(3) | 1.0967(8) | 1.6758(8) | 2.2055(7) |
| 2 | 0.2289(2) | 0.1488(6) | 0.1145(6) | 0.1408(5) |
| 3 | −0.014 03(4) | −0.026 84(12) | −0.029 90(12) | −0.026 09(10) |
| 4 | 0.001 87(5) | 0.002 94(7) | 0.003 97(7) | 0.003 94(6) |

Table XV. Resulting parameters of the polynomial fit to the one dimensional cut through the parity violating potential due to $\langle\gamma^5\rangle$ along the dimensionless reduced normal coordinate ($q_5$) corresponding to the C–Cl stretching mode for the ($S$)-enantiomer of CHBrClF. The standard uncertainties resulting from the fit procedure are given in parenthesis in units of the last preceeding one or two digits.

| $k$ | $c_{\gamma^5,k} \times 10^9$ | | | $c_{\mathrm{ew},k} \times 10^{18}/E_\mathrm{h}$ | | |
|---|---|---|---|---|---|---|
| | HF | B3LYP | LDA | HF | B3LYP | LDA |
| 0 | −1.990(9) | −8.467(9) | −12.361(10) | −6.6223(6) | −1.7856(13) | 2.4332(11) |
| 1 | 2.262(9) | 6.960(9) | 8.746(11) | −1.3870(6) | −1.7214(13) | −2.2413(12) |
| 2 | −0.365(6) | −1.393(7) | −2.026(8) | 0.5257(5) | 0.8027(10) | 0.9370(9) |
| 3 | −0.1313(13) | −0.1378(14) | −0.1432(16) | 0.010 53(9) | −0.0104(2) | −0.025 41(17) |
| 4 | −0.0141(7) | −0.0065(8) | −0.0021(9) | 0.000 72(5) | −0.000 80(11) | −0.001 66(10) |

Table XVI. Resulting parameters of the polynomial fit to the one dimensional cut through the parity violating potential due to $\langle\gamma^5\rangle$ along the dimensionless reduced normal coordinate ($q_6$) corresponding to the C–Br stretching mode for the ($S$)-enantiomer of CHBrClF. The standard uncertainties resulting from the fit procedure are given in parenthesis in units of the last preceeding one or two digits.

| $k$ | $c_{\gamma^5,k} \times 10^9$ | | | $c_{\mathrm{ew},k} \times 10^{18}/E_\mathrm{h}$ | | |
|---|---|---|---|---|---|---|
| | HF | B3LYP | LDA | HF | B3LYP | LDA |
| 0 | −1.992(10) | −8.470(10) | −12.363(12) | −6.6221(2) | −1.7855(2) | 2.433 18(18) |
| 1 | −0.386(10) | −7.319(10) | −9.132(13) | 1.2360(2) | 2.4533(2) | 3.367 77(19) |
| 2 | −0.524(8) | 0.473(7) | 1.205(9) | −0.097 17(15) | −0.309 38(16) | −0.448 57(14) |
| 3 | −0.1653(16) | −0.1497(15) | −0.2089(19) | 0.007 99(3) | 0.019 88(3) | 0.027 30(2) |
| 4 | 0.0293(9) | 0.0276(9) | 0.0295(11) | −0.000 858(17) | −0.001 350(19) | −0.001 481(16) |

Table XVII. Resulting parameters of the polynomial fit to the one dimensional cut through the parity violating potential due to $\langle \boldsymbol{\gamma}^5 \rangle$ along the dimensionless reduced normal coordinate ($q_7$) corresponding to the Cl–F deformation mode for the ($S$)-enantiomer of CHBrClF. The standard uncertainties resulting from the fit procedure are given in parenthesis in units of the last preceeding one or two digits.

| $k$ | $c_{\boldsymbol{\gamma}^5,k} \times 10^9$ | | | $c_{\mathrm{ew},k} \times 10^{18}/E_\mathrm{h}$ | | |
|---|---|---|---|---|---|---|
| | HF | B3LYP | LDA | HF | B3LYP | LDA |
| 0 | −2.01(2) | −8.4670(10) | −12.3597(9) | −6.616(10) | −1.785 58(10) | 2.433 13(13) |
| 1 | −1.07(2) | −6.3547(10) | −8.7064(10) | 5.107(10) | 6.285 21(10) | 6.966 44(13) |
| 2 | 0.238(15) | 0.3690(7) | 0.5143(7) | −0.101(7) | −0.143 52(8) | −0.184 91(9) |
| 3 | 0.004(3) | −0.026 79(15) | −0.047 16(14) | −0.0102(15) | −0.002 693(16) | −0.002 471(19) |
| 4 | −0.0064(18) | 0.005 15(8) | 0.007 98(8) | 0.0031(9) | −0.000 465(9) | −0.000 679(11) |

Table XVIII. Resulting parameters of the polynomial fit to the one dimensional cut through the parity violating potential due to $\langle \boldsymbol{\gamma}^5 \rangle$ along the dimensionless reduced normal coordinate ($q_8$) corresponding to the Br–F deformation mode for the ($S$)-enantiomer of CHBrClF. The standard uncertainties resulting from the fit procedure are given in parenthesis in units of the last preceeding one or two digits.

| $k$ | $c_{\boldsymbol{\gamma}^5,k} \times 10^9$ | | | $c_{\mathrm{ew},k} \times 10^{18}/E_\mathrm{h}$ | | |
|---|---|---|---|---|---|---|
| | HF | B3LYP | LDA | HF | B3LYP | LDA |
| 0 | −1.991(3) | −8.4668(14) | −12.3594(13) | −6.6223(2) | −1.785 58(8) | 2.433 15(17) |
| 1 | −3.607(3) | −23.9595(15) | −34.0517(14) | 6.2705(3) | 9.427 43(9) | 11.474 90(18) |
| 2 | 0.145(2) | −0.3118(11) | −0.6932(10) | 0.0645(2) | 0.187 96(6) | 0.262 09(13) |
| 3 | −0.0438(4) | −0.0525(2) | −0.0622(2) | 0.008 59(4) | 0.011 728(13) | 0.011 03(2) |
| 4 | −0.0027(2) | −0.006 79(12) | −0.008 16(12) | 0.000 30(2) | 0.000 867(7) | 0.001 026(15) |

Table XIX. Resulting parameters of the polynomial fit to the one dimensional cut through the parity violating potential due to $\langle \boldsymbol{\gamma}^5 \rangle$ along the dimensionless reduced normal coordinate ($q_9$) corresponding to the Br–Cl deformation mode for the ($S$)-enantiomer of CHBrClF. The standard uncertainties resulting from the fit procedure are given in parenthesis in units of the last preceeding one or two digits.

| $k$ | $c_{\boldsymbol{\gamma}^5,k} \times 10^9$ | | | $c_{\mathrm{ew},k} \times 10^{18}/E_\mathrm{h}$ | | |
|---|---|---|---|---|---|---|
| | HF | B3LYP | LDA | HF | B3LYP | LDA |
| 0 | −1.989(3) | −8.4665(7) | −12.361(3) | −6.622 21(13) | −1.785 57(10) | 2.433 03(11) |
| 1 | 5.626(3) | 11.2115(7) | 14.674(3) | −1.417 17(13) | −1.896 17(11) | −2.096 90(11) |
| 2 | −0.101(2) | 0.0695(5) | 0.120(2) | −0.014 21(9) | −0.005 04(8) | 0.006 51(8) |
| 3 | −0.0258(4) | −0.022 75(10) | −0.0379(5) | −0.003 510(19) | −0.004 501(16) | −0.004 706(16) |
| 4 | 0.0008(2) | 0.001 27(6) | 0.0008(3) | −0.000 057(11) | −0.000 220(9) | −0.000 331(9) |
